# Supplementary material for: Faster Reinforcement Learning Using Active Simulators
Source: arXiv:1703.07853 source file (2017-11-21)
Supplement: Supplementary file 1 [file appendix.tex]

\section{Appendix}
\label{APPENDIX}

\noindent\textbf{RL algorithms}: A discounted Markov Decision Process (MDP) $\mathcal{M}$ is a tuple $\{\mathcal{S}, \mathcal{A}, \mathcal{P}, \mathcal{R}, \gamma\}$ where $\mathcal{S}$ is the state space, $\mathcal{A}$ is the action space, $\mathcal{P}$ is the state transition probability measure: $\mathcal{P}_{ss'}^a = P[S_{t+1} = s'|S_t = s, A_t = a]$, $\mathcal{R}$ is the state-action reward measure: $\mathcal{R}_{s}^a = E[R_{t+1}|S_t = s, A_t = a]$ and $\gamma$ is the discount factor. A policy $\pi$ is a probability measure of performing an action in a particular state: $\pi[a|s] = P[A_t = a | S_t = s]$. Given an MDP $\mathcal{M}$ and a policy $\pi$, action-value function $q_{\pi}(s,a)$ is defined as the expected total return starting from state $s \in \mathcal{S}$, taking action $a \in \mathcal{A}$ and then following policy $\pi$. From the Bellmann's expectation equation, it follows that:
$ q_{\pi}(s,a) = \mathcal{R}_s^a + \gamma\sum_{s'\in \mathcal{S}}\mathcal{P}_{ss'}^a\sum_{a'\in \mathcal{A}}\pi(a'|s')q_{\pi}(s',a') $.
Optimal action-value function $q_*(s,a)$ is $\max_{\pi}q_{\pi}(s,a)$ and optimal policy $\pi^*$ is given by:
\[ \pi^*(a|s) = \begin{cases} 
      1 & \textrm{if } a = \argmax_{a'\in \mathcal{A}}q_*(s,a') \\
      0 & \textrm{otherwise.} 
   \end{cases}
\]
Using the Bellmann's optimality equation, we get:
$ q_{*}(s,a) = \mathcal{R}_s^a + \gamma\sum_{s'\in \mathcal{S}}\mathcal{P}_{ss'}^a\max_{a'\in \mathcal{A}}q_{*}(s',a') $. This equation is non-linear and many solutions to solve this exist in the literature \emph{e.g.}\ Value Iteration, Policy Iteration, SARSA, \emph{Q}-learning etc (see ~\cite{sutton1998reinforcement} for review). The last two methods are especially applicable when the dynamics and the reward functions are not known in advance (i.e., the RL setting). In our experiments, we demonstrate the validity of our online curriculum learning methods assuming that the RL agent is using the \emph{Q}-learning\cite{watkins1992q} algorithm (this is only for convenience, and any other RL algorithm could be also used). \\

\noindent\textbf{Domain knowledge}: The domain knowledge for a task is represented as a vector of features $F = [F_1, F_2,\ldots, F_n]$, where each $F_i$ characterizes some aspect of the task [\tj{If possible, change these to lower case as long as it does not conflict with notation elsewhere}]. Such vectors can be hand designed by an expert (for instance see~\cite{sinapov2015learning}) and will be assumed given in the domain aware setting of our paper. We will approximate the similarity between two tasks  using a pre-defined notion of similarity of their corresponding feature vectors (for instance, the inverse of their Euclidean distance). Using these feature vectors of the different training tasks, \cite{sinapov2015learning} show that a transfer model can be learned. In our algorithms, we extend this procedure by using tools from active learning to select next tasks in the curriculum. In particular, we use the active linear regression model. [\tj{experimental backing missing, but I think that is okay}]\\

%\noindent\textbf{Diversity measure for tasks}: %Given the features of a pair of tasks - how can we measuring the dissimilarity of the pair.
